# Supplementary material for: FoVolNet: Fast Volume Rendering using Foveated Deep Neural Networks
Source: arXiv:2209.09965 source file (2022-09-20)
Supplement: Supplementary file 1 [file supplemental.tex]

\section{Tabular Data}
All source data tables used to create the analyses and charts in this paper are open and released as a separate archive. All timings for different pipeline components were recorded in milliseconds using the \verb|std::chrono::high_resolution_clock| struct found in the C++ standard library \verb|<chrono>|. Quality measurements where done using Python's \verb|scikit-image| library. We used a custom python implementation to compute MSSSIM. The data is orgnaized as follows.

\begin{itemize}
    \item \verb|cmax|---Compression analysis of our rendering method.
    \item \verb|precision|---Timing data at different model precisions.
    \item \verb|quality|---Quality metrics for FoVolNet and direct prediction at different quality settings. Data was recorded with clips looping. We truncate the data to contain 128 rows of data which provides context around the two 50-frame clips we analyzed.
    \begin{itemize}
        \item All \verb|"*_01"| files have $P_b=0.01$
        \item All \verb|"*_03"| files have $P_b=0.03$
        \item All \verb|"*_07"| files have $P_b=0.07$
        \item All \verb|"*_10"| files have $P_b=0.10$
    \end{itemize}
    \item \verb|throughput|---Timings for each dataset using different methods and different quality settings.
    \begin{itemize}
        \item All \verb|"*_hifi"| files have $P_b=0.07$, $\sigma=0.06$
        \item All \verb|"*_fast"| files have $P_b=0.03$, $\sigma=0.02$
        \item All \verb|"*_ovr"| files use the baseline ray marching renderer.
    \end{itemize}
\end{itemize}

\section{Model Precision}

In addition to qualitative differences, changing the model precision also has effects on the run time. Ideally, the performance gained by reducing precision is inversely proportional to the forfeited accuracy. For example, going from fp32 to fp16 would yield a two times faster run time. Similarly, int8 should offer a four times higher performance when compared to fp32. 

\begin{figure}[!htb]
  \centering
  \includegraphics[width=1.0\columnwidth]{images/supplemental/precision_timings.pdf}
    \caption{Inference speeds for different precisions of the reconstruction network. Data represents averages from a 500-frame long run. Error bars indicate one standard deviation.}
  \label{fig:sup:precision}
\end{figure}

In practice, we do not fully reach these factors due to the way the network is quantized. Some parts cannot be reduced to int8, resulting in a mixed precision network. As shown in Figure~\ref{fig:sup:precision}, int8 quantization achieves between two to three times speedup. 

\section{Eye Tracking}
Foveated rendering requires a way to determine the focal point on the screen. In this project, we used a Tobii Eye Tracker~\cite{Tobii} which allows us to track the user's focal point on the screen in front of them. This data is used to position the high-density foveated area in the rendering.

\section{Image Quality}
We provide high-resolution versions of the image quality matrix from the main document here in Figures~\ref{fig:sup:matrix1} and~\ref{fig:sup:matrix2}.

\begin{figure*}[b]
  \centering
  \includegraphics[width=1.0\textwidth]{images/supplemental/matrix1.pdf}
    \caption{Enlarged version of visual comparison of reconstruction quality using our method. For each dataset, we show the area around the fovea in blue and a part of the periphery in red. All images were generated with $P_b = 0.03$ and $\sigma = 0.02$ for $P_f$.}
  \label{fig:sup:matrix1}
\end{figure*}

\begin{figure*}[b]
  \centering
  \includegraphics[width=1.0\textwidth]{images/supplemental/matrix2.pdf}
    \caption{Enlarged version of visual comparison of reconstruction quality using our method. For each dataset, we show the area around the fovea in blue and a part of the periphery in red. All images were generated with $P_b = 0.03$ and $\sigma = 0.02$ for $P_f$.}
  \label{fig:sup:matrix2}
\end{figure*}
